# Supplementary material for: Constructive Discrepancy Minimization with Hereditary L2 Guarantees
Source: arXiv:1711.02860 source file (2018-12-13)
Supplement: Supplementary file 1 [file appendix.tex]

\section{Missing Proofs}
In this section, we give the missing proofs of the following two results from Section~\ref{sec:algo}:

\begin{customlem}
{\ref{lem:smallmax}}
The \textbf{PartialColor} algorithm satisfies that:
$$\Pr[\max_i |\hat{x}_i| > 1]  = k^{-\Omega(1)}.$$
\end{customlem}

\begin{customlem}
{\ref{lem:fewlive}}
The \textbf{PartialColor} algorithm satisfies that there are no more
than $k/2$ live coordinates in $\hat{x} = x+\gamma$ with probability
at least $7/8$.
\end{customlem}

\paragraph{No Large Coordinates.}
The first thing we bound is the probability that there is some
coordinate $i$ of $\hat{x}$ with $|\hat{x}_i| > 1$ (proof of Lemma~\ref{lem:smallmax}). The main idea in
the proof follows previous work quite closely. More concretely, we
observe that as soon as a coordinate exceeds $1-\delta$ in absolute value, it will never
change again. Thus for a coordinate to exceed $1$, it must be the case
that adding a single vector $\eps v$ to $\gamma$ caused a coordinate
to increase by at least $\delta$ in absolute value. Since $\eps$ is
sufficiently smaller than $\delta$ and our vectors $v$ are sampled
from a fairly high-dimensional subspace, this will happen with tiny
probability. We are ready for the formal proof.

We start by proving that no coordinate of $\gamma$ changes by much when
adding $\eps v$ to $\gamma$ in step (e) of the algorithm. More formally, we prove:
\begin{lemma}
\label{lem:deviate}
For any parameter $\lambda > 0$, we have:
$$
\Pr\left[ \max_j \max_i |\langle V_j, e_i \rangle| > \lambda\right] \leq 2kT\exp(-\lambda^2/2).
$$
\end{lemma}

\begin{proof}
Consider any $e_i$ and any $V_j$. If $e_i$ is not live in the $j$'th
iteration of the for-loop, then $\langle V_j , e_i \rangle = 0$ since
we choose $V_j$ in a subspace orthogonal to $e_i$. Thus the rest of
the analysis assumes $i$ is live during the $j$'th iteration. Note
that there are at most $k$ such indices $i$. We have:
\begin{eqnarray*}
\langle V_j , e_i \rangle &=& \langle \sum_{h=n-k/4+1}^n G_{j,h}
Q_{j,h}, e_i \rangle \\
&=& \sum_{h=n-k/4+1}^n G_{j,h} \langle 
Q_{j,h}, e_i \rangle.
\end{eqnarray*}
If the algorithm already terminated in (a) in the $j$'th iteration or
earlier, we have $G_{j,h}=0$ for all $h$ and thus 
$$
\Pr\left[ |\max_i \langle V_j, e_i \rangle| > \lambda\right] = 0 < 2\exp(-\lambda^2/2).
$$
Otherwise, each $G_{j,h}$ is $\Norm(0,1)$ distributed and we see that:
\begin{eqnarray*}
\langle V_j , e_i \rangle &\sim& \Norm\left(0, \sum_{h=n-k/4+1}^n \langle 
Q_{j,h}, e_i \rangle^2\right).
\end{eqnarray*}
But $\sum_{h=n-k/4+1}^n \langle 
Q_{j,h}, e_i \rangle^2$ is the squared $\ell_2$-norm of the length of
the projection of $e_i$ onto $\spn(Q_{j,n-k/4+1},\dots,Q_{n})$. Since
this is no more than $\|e_i\|_2^2 = 1$, we have that
$$
\Pr[|\langle V_j , e_i \rangle| \geq \lambda] \leq 2\exp(-\lambda^2/2).
$$
By a union bound over all $e_i$ that were live when we started the
partial coloring and over all $j$, we get that
$$
\Pr[\max_j \max_i |\langle V_j , e_i \rangle| \geq \lambda] \leq
2kT\exp(-\lambda^2/2). 
$$
\end{proof}

\begin{corollary}
\label{cor:deviate}
For any parameter $\lambda > 0$, we have:
$$
\Pr\left[ \max_i |\hat{x}_i| > 1-\delta + \lambda\right] \leq
2kT\exp(-\eps^{-2} \lambda^2/2).
$$
\end{corollary}

\begin{proof}
Assume $\max_j \max_i |\langle V_j ,e_i \rangle | \leq \lambda$ for
some $\lambda > 0$ and consider a coordinate $i$. Since our algorithm
always chooses a $v$ such that $v$ is orthogonal to all $e_j$ with $j
\in S$, it follows that $\langle V_j, e_i \rangle$ is non-zero only if
$|(x + \gamma)_i| < 1-\delta$ when reaching iteration $j$. This
implies that, conditioned on  $\max_j \max_i |\langle V_j ,e_i
\rangle | \leq \lambda$, we always have $|(x + \gamma)_i| < 1-\delta + \eps
\lambda$ since we
add $\eps v$ to $\gamma$ in step (e). Substituting $\lambda$ by $\eps^{-1}
\lambda$ in Lemma~\ref{lem:deviate} completes the proof.
\end{proof}

It follows immediately from Corollary~\ref{cor:deviate} that
\begin{eqnarray*}
\Pr[\max_i |\hat{x}_i| > 1] &\leq& 2kT\exp(-\eps^{-2} \delta^2/2) \\
&=& 2kT\exp(-c_0 (\ln(k/\delta)/\delta^2) \delta^2/2) \\
&=& 2kT k^{-c_0/2} \delta^{c_0} \\
&=& k^{-\Omega(1)}.
\end{eqnarray*}
Thus we have proved Lemma~\ref{lem:smallmax}.

\paragraph{Rarely Aborts.}
In this paragraph, we prove that \textbf{PartialColor} most often
terminates in step (a) rather than aborting in step 6. When it terminates in
(a), we have that there are no more than $k/2$ live coordinates in
$\hat{x} = x + \gamma$, which is what we want to prove in Lemma~\ref{lem:fewlive}. The main idea in our proof is to show that
$\E[\|\sum_{j=1}^T V_j \|_2^2]$ is very large if the probability of
returning in step (a) is small. Combining this with the fact that all
coordinates of $\hat{x}$ are bounded by $1$ with high probability
gives a contradiction and thus we must have that we often terminate in
step (a). We start by bounding $\E[\|\sum_{j=1}^T V_j \|_2^2]$:
\begin{eqnarray*}
\E\left[ \|\sum_{j=1}^{T} V_j\|_2^2\right] &=& \E\left[ \left(\sum_{j=1}^{T}
  V_j\right)^T\left(\sum_{j=1}^{T}
  V_j \right)\right]  \\
&=& \sum_{j=1}^T\E\left[ \|V_j\|_2^2\right] + \sum_{j=1}^T \sum_{h \neq j}
\E\left[\langle V_j, V_h \rangle \right] \\
&=&\sum_{j=1}^T \sum_{i=n-k/4+1}^n \E \left[ G_{j,i}^2\right]  + \sum_{j=1}^T \sum_{h \neq j}
\E\left[\langle V_j, V_h \rangle \right]
\end{eqnarray*}
To analyse $\E \left[ G_{j,i}^2\right]$, let $E_j$ denote the event
that the algorithm already terminated in step (a) in some iteration $i
\leq j$ of the for-loop. Then 
\begin{eqnarray*}
\E \left[ G_{j,i}^2\right] &=& \Pr[E_j]\E \left[ G_{j,i}^2 \mid E_j
\right] + (1-\Pr[E_j]) \E \left[ G_{j,i}^2 \mid \neg E_j
\right] \\
&=& \Pr[E_j] \cdot 0 +  (1-\Pr[E_j]) \cdot 1 \\
&=& (1-\Pr[E_j]).
\end{eqnarray*}
We thus have:
\begin{eqnarray*}
\E\left[ \|\sum_{j=1}^{T} V_j\|_2^2\right] &=&  \sum_{j=1}^Tk(1-\Pr[E_j])/4 + \sum_{j=1}^T \sum_{h \neq j}
\E\left[\langle V_j, V_h \rangle \right] \\
&=& (k/4)\sum_{j=1}^T(1-\Pr[E_j]) + \sum_{j=1}^T \sum_{h \neq j}
\sum_{i=n-k/4+1}^n \sum_{\ell=n-k/4+1}^n \E\left[G_{j,i} G_{h,\ell}\langle Q_{j,i}, Q_{h,\ell} \rangle \right] \\
\end{eqnarray*}
Consider $\E\left[G_{j,i} G_{h,\ell}\langle Q_{j,i}, Q_{h,\ell} \rangle
\right]$ and assume wlog. that $j > h$. Then for any values $g \in \supp(G_{h,\ell}),
q_1 \in \supp(Q_{j,i})$ and $q_2 \in \supp(Q_{h,\ell})$,  the random variable $G_{j,i}$ is still symmetric around
zero when conditioning on $G_{h,\ell}=g \wedge Q_{j,i}=q_1 \wedge
Q_{h,\ell}=q_2$. Hence $\E[G_{j,i} G_{h,\ell}\langle Q_{j,i}, Q_{h,\ell}
\rangle ] = 0$ and we conclude:
$$
\E\left[ \|\sum_{j=1}^T V_j \|_2^2\right] =  (k/4)\sum_{j=1}^T(1-\Pr[E_j]).
$$
Now define $M_r$ as the event $\max_i |\hat{x}_i| \in (r, r+1]$ for
every integer $r > 0$. Define $M_0$ as the event $\max_i |\hat{x}_i|
\leq 1$. We have:
\begin{eqnarray*}
\E\left[ \|\sum_{j=1}^T V_j \|_2^2\right]  =
\Pr[M_0] \cdot \E\left[ \|\sum_{j=1}^T V_j \|_2^2 \mid
 M_0 \right] + \sum_{r=1}^{\infty} \Pr[M_r]\cdot \E\left[ \|\sum_{j=1}^T V_j \|_2^2 \mid
M_r \right].
\end{eqnarray*}
We now use that conditioned on $M_r$, we have all coordinates
of $\sum_{j=1}^T V_j$ bounded by $\eps^{-1}(1-\delta + r+1) <
\eps^{-1}(r+2)$. To see this, note that we
start out with $|x_i| < 1-\delta$ for all $i$ and $M_r$ says that
$\max_i |\hat{x}_i| < r+1$. But $\hat{x}_i = x_i + (\sum_j \eps
V_j)_i$ and thus all coordinates are bounded as claimed. Moreover, there are at most $k$ non-zero coordinates
of $V_j$ (since there are no more than $k$ live coordinates and $V_j$
is orthogonal to all $e_i$ where $i$ is not live).
This implies that $\|\sum_{j=1}^T V_j
\|_2^2 \leq k\eps^{-2}(r+2)^2$. Using Corollary~\ref{cor:deviate} to bound
$\Pr[M_r]$ for $r>0$, we get that
\begin{eqnarray*}
\E\left[ \|\sum_{j=1}^T V_j \|_2^2\right]  &\leq& \\
\Pr[M_0] \cdot 4\eps^{-2}k + \sum_{r=1}^{\infty} 2kT \exp(-\eps^{-2} (r+1)^2/2)
k\eps^{-2}(r+2)^2  &=& \\
\Pr[M_0] \cdot 4\eps^{-2}k + \sum_{r=1}^{\infty} 240 k^2 \exp(-\eps^{-2} (r+1)^2/2)
\eps^{-4}(r+2)^2.
\end{eqnarray*}
Since $\eps^{-2} \geq c_0 \ln
k$ for a big enough constant $c_0$, we get
\begin{eqnarray*}
\E\left[ \|\sum_{j=1}^T V_j \|_2^2\right]  \leq \Pr[M_0] \cdot 4\eps^{-2}k +1 
\leq 4\eps^{-2}k+1.
\end{eqnarray*}
We have thus shown that
$$
4\eps^{-2}k+1 \geq (k/4)\sum_{j=1}^T(1-\Pr[E_j]).
$$
Since $\Pr[E_j] \geq \Pr[E_h]$ for $j > h$, we get that
\begin{eqnarray*}
4\eps^{-2}k+1 \geq (k/4)T(1-\Pr[E_T]) \Rightarrow \\
(1-\Pr[E_T]) \leq \frac{16 \eps^{-2}k+4}{kT} \Rightarrow \\
\Pr[E_T] \geq 1-\frac{16 \eps^{-2}k+4}{kT} \geq 1-\frac{20 \eps^{-2}k}{kT}.
\end{eqnarray*}
Since $T = 160 \eps^{-2}$, we get that $\Pr[E_T]
\geq 7/8$. We have thus proved Lemma~\ref{lem:fewlive}.
